# Supplementary material for: Observation of $e^+e^-\to\omega\chi_{bJ}(1P)$ and search for $X_b \to \omega\Upsilon(1S)$ at $\sqrt{s}$ near 10.75 GeV
Source: arXiv:2208.13189 source file (2023-01-29)
Supplement: Supplementary file 1 [file Supplemental_Material.pdf]

# Supplemental Material

## Two-dimensional distributions of $M(\pi^+\pi^-\pi^0)$ versus $M(\gamma\Upsilon(1S))$

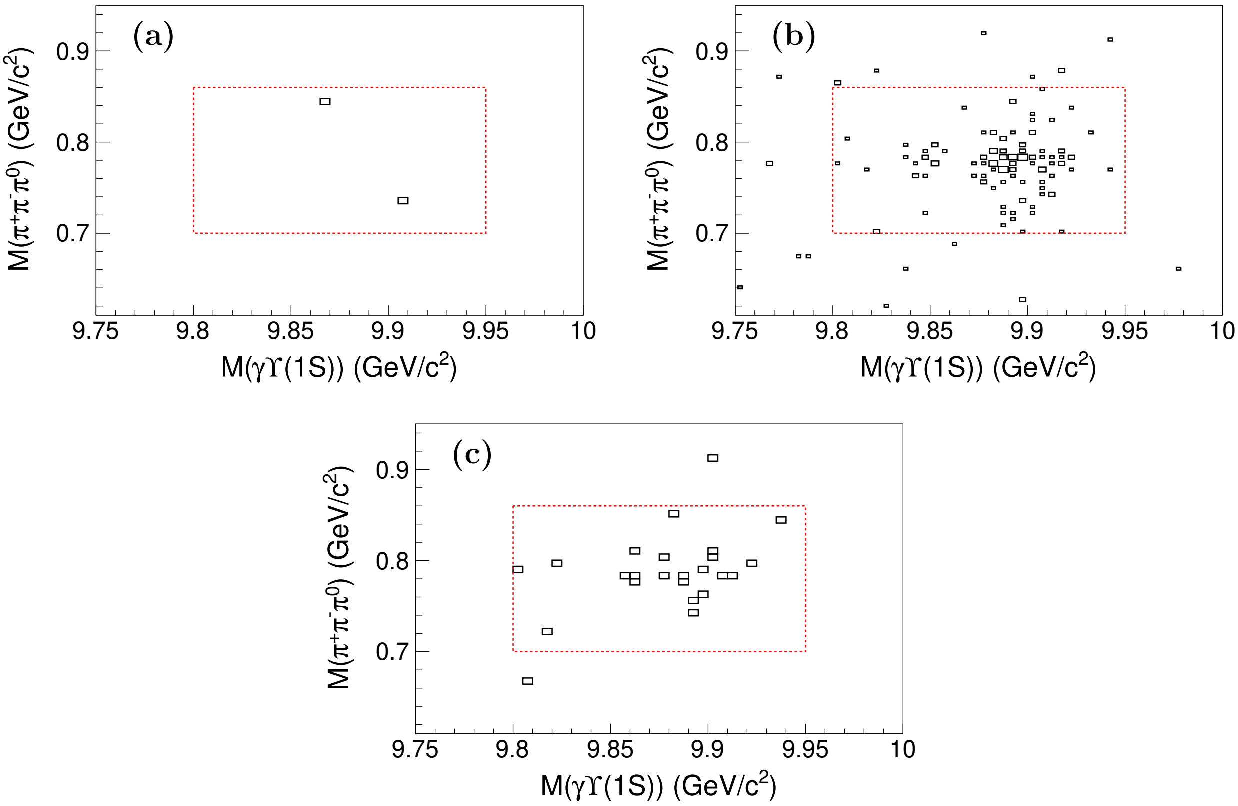


FIG. 1: Two-dimensional mass distributions of $M(\pi^+\pi^-\pi^0)$ versus $M(\gamma\Upsilon(1S))$ at $\sqrt{s}$ = (a) 10.701, (b) 10.745, and (c) 10.805 GeV, respectively. The red dashed boxes show the $\omega$ and $\chi_{bJ}$ signal regions, where more than 90% signal events are retained according to signal MC simulations.

## Inputs and upper limits obtained for $X_b$ masses from 10.45 to 10.65 GeV/$c^2$

TABLE I: Inputs and upper limits obtained for $X_b$ masses from 10.45 to 10.65 GeV/$c^2$ (at 90% Bayesian credibility) on the product of cross section times branching fraction $\sigma_B^{\rm UL}(e^+e^- \to \gamma X_b)\mathcal{B}(X_b \to \omega\Upsilon(1S))$ ($\sigma_{X_b}^{\rm UL}$) at $\sqrt{s}$ = 10.653, 10.701, 10.745, and 10.805 GeV. Since the upper limits depend on the test $X_b$ mass, only the least stringent bounds are reported for each collision energy.

| $\sqrt{s}$ (GeV) | $M_{X_b}$ (GeV/$c^2$) | $N^{\rm UL}$ | $\varepsilon$ | $\lvert 1-\Pi\rvert^2$ | $1+\delta_{\rm ISR}$ | Syst (%) | $\sigma_{X_b}^{\rm UL}$ (pb) |
|---|---|---|---|---|---|---|---|
| 10.653 | 10.59 | 10.0 | 0.154 | 0.931 | 0.72 | 8.7 | 0.55 |
| 10.701 | 10.45 | 8.1 | 0.166 | 0.931 | 0.76 | 8.7 | 0.84 |
| 10.745 | 10.45 | 8.1 | 0.164 | 0.931 | 0.78 | 8.7 | 0.14 |
| 10.805 | 10.53 | 10.7 | 0.165 | 0.932 | 0.81 | 8.8 | 0.37 |

# Fractional systematic uncertainties (%) in the measurements of $\sigma_B(e^+e^- \to \omega\chi_{bJ})$ and $\sigma_B(e^+e^- \to \gamma X_b)\mathcal{B}(X_b \to \omega\Upsilon(1S))$

TABLE II: Fractional systematic uncertainties (%) in the measurements of $\sigma_B(e^+e^- \to \omega\chi_{bJ})$ and $\sigma_B(e^+e^- \to \gamma X_b)\mathcal{B}(X_b \to \omega\Upsilon(1S))$. Systematic uncertainties from detection efficiency, branching fractions, trigger, and luminosity are correlated between various energy points while other systematic uncertainties are uncorrelated.

| Final states | $\omega\chi_{b0}/\omega\chi_{b1}/\omega\chi_{b2}$ | | | $\gamma X_b$ | | | |
|---|---|---|---|---|---|---|---|
| $\sqrt{s}$ (GeV) | 10.701 | 10.745 | 10.805 | 10.653 | 10.701 | 10.745 | 10.805 |
| Detection efficiency | 7.2 | 7.2 | 7.2 | 7.2 | 7.2 | 7.2 | 7.2 |
| Branching fractions | 14.7/7.4/7.3 | 14.7/7.4/7.3 | 14.7/7.4/7.3 | 4.7 | 4.7 | 4.7 | 4.7 |
| Radiative correction factor | 2.0 | 5.1 | 13.7 | 0.2 | 0.4 | 0.5 | 0.7 |
| Angular distribution | 1.0 | 1.0 | 1.0 | 1.0 | 1.0 | 1.0 | 1.0 |
| Fit model | - | 16.3/4.6/8.2 | 10.9/8.9/20.0 | - | - | - | - |
| Trigger | 1.0 | 1.0 | 1.0 | 1.0 | 1.0 | 1.0 | 1.0 |
| Beam energy | - | 10.5/2.5/3.0 | 6.5/5.0/12.2 | - | - | - | - |
| Luminosity | 0.6 | 0.6 | 0.6 | 0.6 | 0.6 | 0.6 | 0.6 |
| Total | 16.6/10.6/10.6 | 25.9/12.7/14.5 | 24.9/20.2/29.1 | 8.7 | 8.7 | 8.7 | 8.8 |
